# Supplementary material for: Enhanced spin-orbit interaction and Kondo scattering in $\delta$-doped LaTiO$_3$/SrTiO$_3$ interfaces
Source: arXiv:1402.1915 source file (2014-08-01)
Supplement: Supplementary file 1 [file Shubhankar__supplementary.pdf]

# Enhanced spin-orbit interaction and Kondo scattering in $\delta$-doped $LaTiO_3/SrTiO_3$ interfaces

Shubhankar Das[1], A. Rastogi[1], Lijun Wu[2], Jin-Cheng Zheng[3], Z. Hossain[1], Yimei Zhu[2] and R. C. Budhani[1,4,*]
[1] *Condensed Matter - Low Dimensional Systems Laboratory, Department of Physics, Indian Institute of Technology, Kanpur 208016, India*
[2] *Condensed Matter Physics and material science department, Brookhaven National Laboratory, Upton, NY 11973, USA*
[3] *Department of Physics and Fujian Provincial Key Laboratory of Theoretical and Computational Chemistry, Xiamen University, Xiamen 361005, China*
[4] *National Physical Laboratory, Council of Scientific and Industrial Research (CSIR), New Delhi - 110012, India*

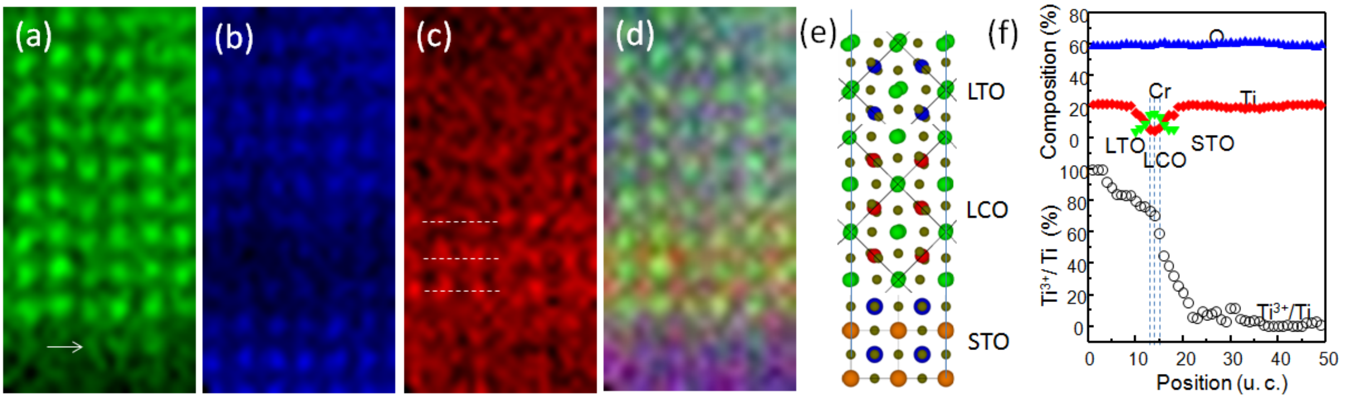


FIG. S1: Two dimensional elemental map of La, Ti and Cr based on EELS spectrum image are shown in the panel (a), (b) and (c) respectively. (d) is the color mixture of (a), (b) and (c). (e) is the atomic projection of the interface with green, blue, red, brown and orange spheres representing La, Ti, Cr, O and Sr respectively. (f) atomic position of O, Ti, and Cr, as well as $Ti^{3+}/Ti$ percentage as a function of probe position.

Fig. S1 reveals that the La layer of $LaCrO_3$ (LCO) grows on the Ti layer of the $SrTiO_3$ (STO). Above the La layer, there are three layers of Cr (indicated by dashed line in Fig. S1(c)). A small amount of La diffuses to neighboring Sr site in STO as indicated by the arrow in Fig. S1(a). Fig. S1(d) color mixture from Fig. S1 (a-c). Fig. S1(e) structure model of STO, LCO, $LaTiO_3$ (LTO) with orange, blue, green and dark yellow spheres representing Sr, Ti, Cr and O respectively. Composition mapping revealed a constant distribution of oxygen across the region and complementary increase and decrease in Cr and Ti, respectively, in the LCO layer with a 1-2 uc diffusion length, based on the FWHM measurements of the elemental intensities, is shown in fig. S1(f). The percentage of $Ti^{3+}$ over the sum of $Ti^{3+}$ and $Ti^{4+}$ (denoted as $Ti^{3+}/Ti$ percebtage) across the interface suggest a significant charge transfer from LTO to STO near the interface.

First principles calculations based on density functional theory (DFT)[1, 2] have been carried out utilizing the Quantum Espresso (QE) package[3] with ultrasoft pseudopotential[4]. In the first principles calculations, the exchange-correlation interaction is described by the Perdew-Burke-Ernzerh of generalized gradient approximation (PBE-GGA)[5], the kinetic energy cutoff is set to 40 Ry for wavefunctions and 400 Ry for charge and potential; converge threshold for self-consistency is proposed to be $10^{-8}$ (a. u.) with $8 \times 8 \times 1$ k grid for Brillouin zone sampling. Supercells containing three unit cells (uc) of LTO, $\delta$ uc of LCO and 3 uc of STO and a vacuum layer are used in the calculation. Different number uc of LCO layer (i. e., $\delta = 0$, 1 and 3 uc) are chosen to examine the effects of thickness of LCO layer on charge transfer of $(LaTiO_3)_3(LaCrO_3)_\delta(SrTiO_3)_3$. The lattices a and b of the supercell are kept the same as that of substrate STO, but the atomic position and c-axis are fully relaxed to optimized geometry. The orbital projected density of states and charge are analyzed by *Löwdin* scheme. The charge transfer of $(LaTiO_3)_3(LaCrO_3)_\delta(SrTiO_3)_3$ is determined by comparing the orbital projected charge of Ti and Cr d orbitals in supercell with bulk counterpart, namely LTO, LCO and STO.

Fig. S2 shows sheet resistance ($R_\square$) vs temperature of $\delta = 5$ uc in zero magnetic field. The solid straight line is a ln T fit in a small temperature range below the resistance minimum. The slope is fairly insensitive to magnetic field.

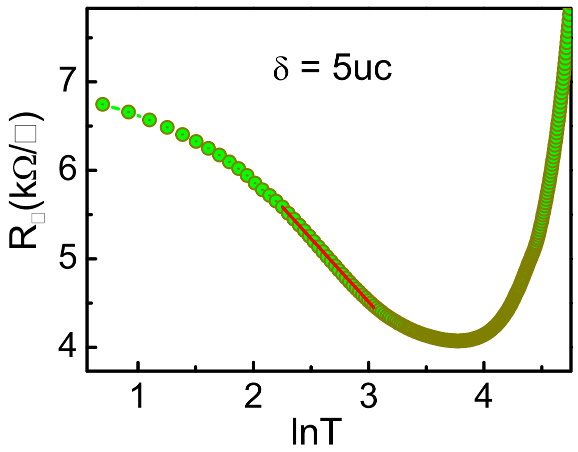


FIG. S2: R□ vs ln T plot of $\delta$ = 5 uc sample at zero magnetic field. The solid straight line is the ln T fit below resistance minimum.

Here the resistance minimum followed by a ln T increase of R□ and then a saturation points toward the Kondo type scattering arising from $S = {}^1\!/_2$ $Ti^{3+}$ ions (for pure LTO/STO sample) and $Ti^{3+}$ ($S = {}^1\!/_2$) and $Cr^{3+}$ ($S = {}^3\!/_2$) both (for LTO/LCO/STO heterostructures).

The positive out-of-plane MR ($MR_\perp$) (Fig. 3 in main text) in these heterostructures may be the result from electron-electron (e-e) interaction and/or classical orbital effect. In the former case, the magnetoconductance goes as $\sim -\frac{e^2}{\hbar}\frac{\tilde{F}_\sigma}{4\pi^2}(0.084) \times \left(\frac{g\mu_B H}{k_B T}\right)^2$ for $\frac{g\mu_B H}{k_B T} \ll 1$, where $\tilde{F}_\sigma$ has the upper bound of 4/3. Now taking the standard value of e, $\hbar$, $\mu_B$, $k_B$ and taking g = 2 (as charge carriers are electron), T = 4.2 K, $\tilde{F}_\sigma = 4/3$ we calculate the slope of MR vs $H^2$ curve is $\approx 0.714 \times 10^{-7}$ /Tesla$(\mathcal{T})^2$ for e-e interaction. But the calculated slope from the experimental data of $\delta = 0$ uc is $1.69 \times 10^{-3}$ $/\mathcal{T}^2$. So, we can conclude that e-e interaction is not the only scattering process for this large $MR_\perp$.

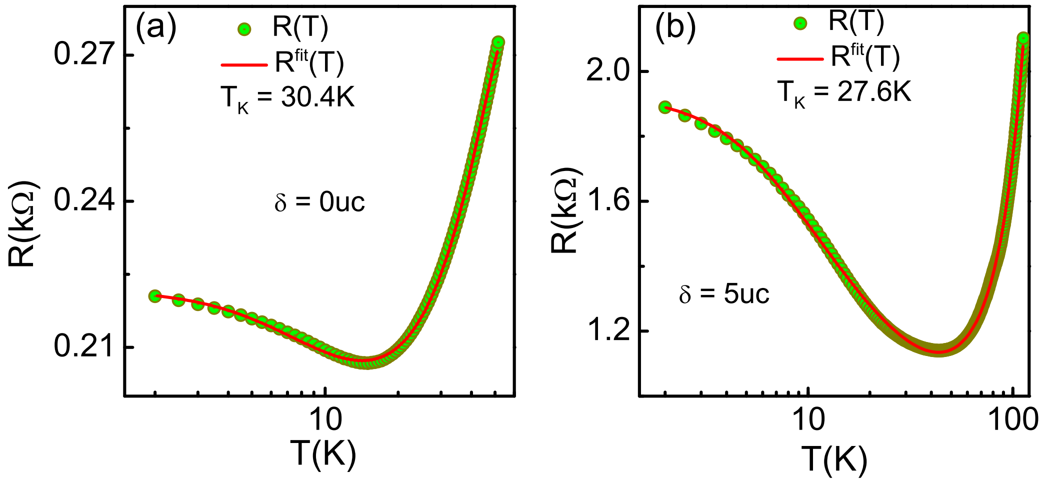


FIG. S3: Longitudinal resistance at H = 0 as a function of temperature for $\delta$ = 0 and 5 uc. Solid curve is a fit using Eq. (1) and (2). This yields $T_K$ = 30.4 K and 27.6 K for $\delta$ = 0 and 5 uc respectively.

The appearance of a saturating resistance at temperature below the resistance minimum is a characteristics feature of the Kondo effect. The contribution of the magnetic impurity to the temperature dependent electrical resistivity is a universal function in units of Kondo temperature ($T_K$). This function $R_K(T/T_K)$ behaves logarithmically at higher temperature $T >> T_K$, and saturates at low temperature, so that $R_K(T/T_K) \approx R_K(0K)(1 - 6.88(T/T_K)^2)$ for

$T \ll T_K$, if we define $T_K$ as the temperature where Kondo resistivity is half of it's zero temperature value[6, 7]. In a temperature range below and above the resistance minimum, resistance can be described by simple Kondo model [8]

$$R^{fit}(T) = R_0 + aT^2 + bT^5 + R_K(T/T_K) \tag{1}$$

where $R_0$ is the residual resistance due to sample disorder, $T^2$ is the e-e interaction term and $T^5$ represents electron-phonon interaction. For fitting of this model to the experimental data, we use an empirical form [8]

$$R_K(T/T_K) = R_K(T=0)\left(\frac{T_K^{'2}}{T^2 + T_K^{'2}}\right)^S \tag{2}$$

where $T_K^{'} = \mathrm{T}_K/(2^{1/S} - 1)^{1/2}$. Fig. S3 (a) and (b) show the temperature dependence resistance of $\delta = 0$ and 5 uc respectively. The solid red line is a fit using Eq. (1) and (2). We choose S = 0.225 to fit the data closely. The fitting parameters for $\delta = 0$ and 5 uc are $\mathrm{R}_0 = 146\ \Omega$, a = 0.04786 $\Omega/K^2$, b = 8.774 $\times\ 10^{-8}\ \Omega/K^5$, $\mathrm{R}_K(0\ \mathrm{K}) = 75\ \Omega$, $\mathrm{T}_K =$ 30.4 K and $\mathrm{R}_0 = 350\ \Omega$, a = 0.07151 $\Omega/K^2$, b = 2.282 $\times\ 10^{-8}\ \Omega/K^5$, $\mathrm{R}_K(0\ \mathrm{K}) = 1574\ \Omega$, $\mathrm{T}_K = 27.6$ K respectively.

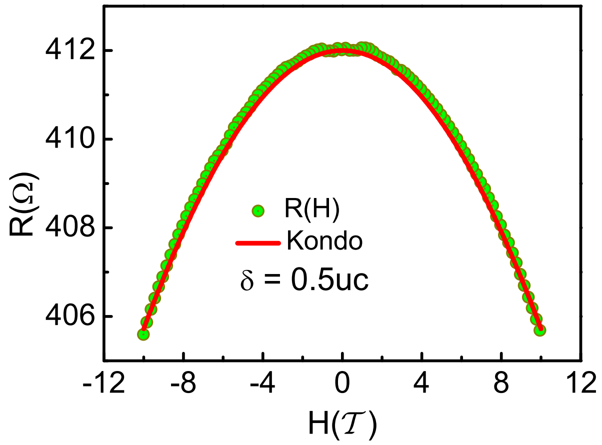


FIG. S4: shows $\mathrm{MR}_{\parallel}$ at 10 K of $\delta = 0.5$ uc. Solid curve: $R^{model}\left(H_{\parallel}\right)$ is a fit according to Eq. (3), (4) and (5) where we choose $R_0 = 226\ \Omega$ and $H_1 = 28.5\ \mathcal{T}$.

To compare the in-plane magnetoresistance ($\mathrm{MR}_{\parallel}$) with the theory, we use the zero temperature Kondo MR expression of Lee et. al. [8]. At zero temperature, a Kondo impurity magnetization is given as [8, 9]

$$M(H/H_1) = \begin{cases} \frac{1}{\sqrt{2\pi}} \sum\limits_{k=0}^{\infty} \left(-\frac{1}{2}\right)^k (k!)^{-1} \left(k+\frac{1}{2}\right)^{\left(k-\frac{1}{2}\right)} e^{-\left(k+\frac{1}{2}\right)} \left(\frac{H}{H_1}\right)^{2k+1}, H \leq \sqrt{2}H_1 \\ 1 - \pi^{-3/2} \int \frac{dt}{t} \sin\left(\pi t\right) e^{-t\ln(t/2e)} \left(\frac{H}{H_1}\right) \Gamma(t+1/2), \sqrt{2}H_1 \leq H \end{cases} \tag{3}$$

where $H_1$ is a magnetic field scale, related to both Kondo temperature and the g-factor of impurity spin. After calculating the magnetization of impurity, the zero temperature Kondo-magnetoresistance is given by

$$R_K\left(H/H_1\right) = R_k\left(H=0\right)\cos^2\left(\frac{\pi}{2}M\left(H/H_1\right)\right) \tag{4}$$

And the $\mathrm{MR}_{\parallel}$ is given by

$$R\left(H_{\parallel}\right) = R_0 + R_k\left(H_{\parallel}/H_1\right) \tag{5}$$

In Fig. S4, the solid red line is a fit with the experimental negative $\mathrm{MR}_{\parallel}$ data at 10 K of $\delta = 0.5$ uc by Eq. (3), (4) and (5). The excellent fit between experimental data and theory points towards Kondo type scattering at low temperatures. In table S1 we have listed the value of $\mathrm{R}_0$ and $\mathrm{H}_1$ for $\delta = 0$, 0.5 and 3 uc.

At T $\leqslant$ 10 K a small positive MR in $\mathrm{H}_{\parallel}$ field followed by transition to the negative MR regime indicates dominant effect of weak anti-localization (WAL) at low temperature. Thus we add the WAL term to the Kondo interaction term in MR equation and it follows as;

$$R\left(H_{\parallel}\right) = R_0 + R_k\left(H_{\parallel}/H_1\right) + a\left[\Psi\left(\frac{1}{2} + \frac{H\varphi}{H_{\parallel}}\right) - \ln\left(\frac{H_{\varphi}}{H_{\parallel}}\right)\right] \tag{6}$$

TABLE S1: Here we have shown the fitting parameters, $R_0$ and $H_1$, for $\delta$ = 0. 0.5 and 3 uc.

| Fitting parameters | $\delta$ = 0 uc | $\delta$ = 0.5 uc | $\delta$ = 3 uc |
|---|---|---|---|
| $R_0$ | 146 Ω | 227 Ω | 289 Ω |
| $H_1$ | 23 $\mathcal{T}$ | 28.5 $\mathcal{T}$ | 22 $\mathcal{T}$ |

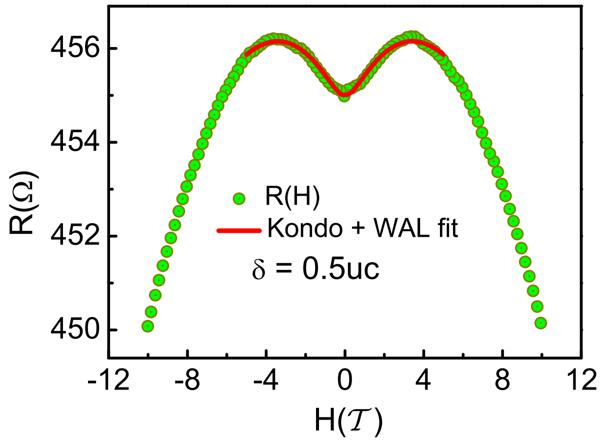


FIG. S5: shows $MR_{||}$ at 2K of $\delta$ = 0.5uc. Solid curve: $R^{model}\left(H_{||}\right)$ is a fit according to Eq. (6)

In Fig. S5 we fit the $MR_{||}$ at 2 K of $\delta$ = 0.5 uc with Eq. (6). It can be seen that our model is consistent with the experimental observations.

The magnetoresistance R(H) - R(H = 0) of the $\delta$ = 0, 0.5 and 3 uc for different orientation ($\theta$) of the magnetic field with respect to sample normal is shown in Fig. S6 (a-c). At $\theta = 90^0$, H is in the film plane but perpendicular to the direction of current. For $H_\perp$ configuration ($\theta$ = 0), all the samples shows positive MR. As we tilt the magnetic field towards sample plane, a crossover from positive MR to negative MR is observed. This change of sign at 2 K and 10 $\mathcal{T}$ happens at $80^0$, $70^0$ and $50^0$ for $\delta$ =0, 0.5 and 3 uc respectively. In the inset of Fig. S6(a-c) the resistance at 2 K and 10 $\mathcal{T}$ as a function of angle $\theta$ is shown. The resistance minimum is observed when the magnetic field is in the plane of the surface. The black line in inset of Fig. S6(a-c) is a fit using $R(\theta, T) = r(T)\cos^2(\theta) + R_0(T)$, where r(T = 2 K) = 33, 36, 44 Ω and $R_0$(T = 2 K) = 233, 466, 906 Ω for $\delta$ = 0, 0.5, 3 uc samples respectively. The origin of two-fold oscillation in anisotropic MR can be from the Lorentz scattering of the charge carriers, which follows the $\cos^2\theta$ dependence. This also suggests the 2-D nature of the electron confinement at the interface.

* Electronic address: `rcb@iitk.ac.in,rcb@nplindia.org`

[1] P. Hohenberg and W. Kohn, Phys. Rev. **136,** B864 (1964).
[2] W. Kohn and L. J. Sham, Phys. Rev. **140,** A1133 (1965).
[3] P. Giannozzi et al., J. Phys. Condens. Matter. **21,** 395502 (2009).
[4] D. Vanderbilt, Phys. Rev. B (Rapid Communications) **41,** 7892 (1990).
[5] J. P. Perdew, k. Burke, and M. Ernzerhof, Phys. Rev. Lett. **77,** 3865 (1996).
[6] J.Kondo, Prog. Theor. Phys. **32,** 37 (1964).
[7] T. A. Costi, Phys. Rev. Lett. **85,** 1504 (2000).
[8] M. Lee et al., Phys. Rev. Lett. **107,** 256601 (2011).
[9] N. Andrei, K. Furuya and J. Lowenstein, Rev. Mod. Phys. **55,** 331 (1983).
[10] T. L. Daulton and B. J. Little, Ultramicroscopy 106, 561 (2006).

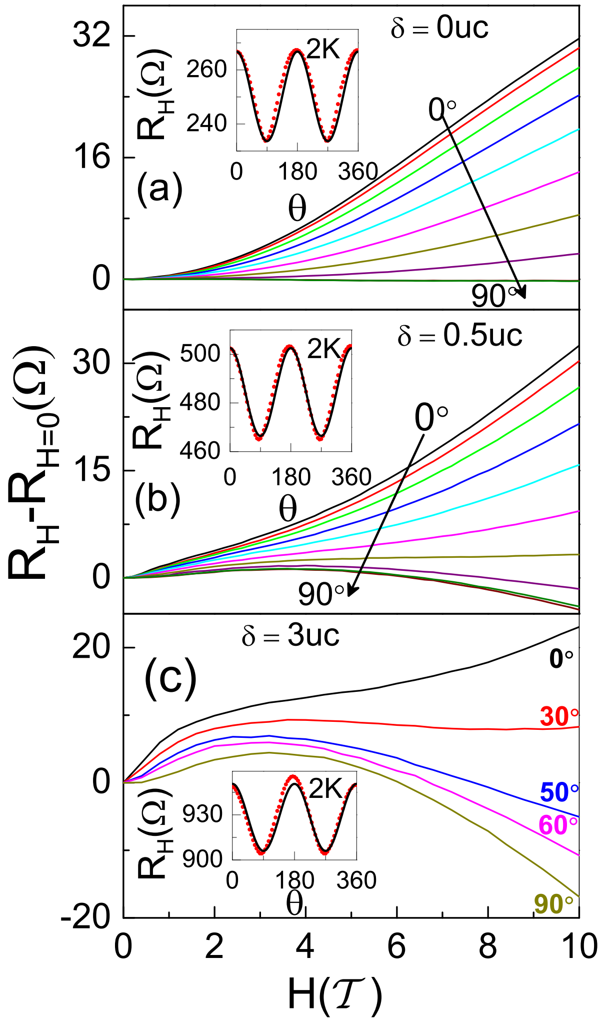


FIG. S6: (a-c) Show MR for different orientation of H with respect to sample plane for $\delta = 0$, 0.5 and 3 uc respectively. Angle $\theta$ is measured from the normal of the sample plane, and $\theta = 90^0$ implies H $\parallel$ sample plane but H $\perp$ $\mathbf{j}$. Insets show angular dependence of resistance at 2 K in 10 $\mathcal{T}$ field for the three samples.

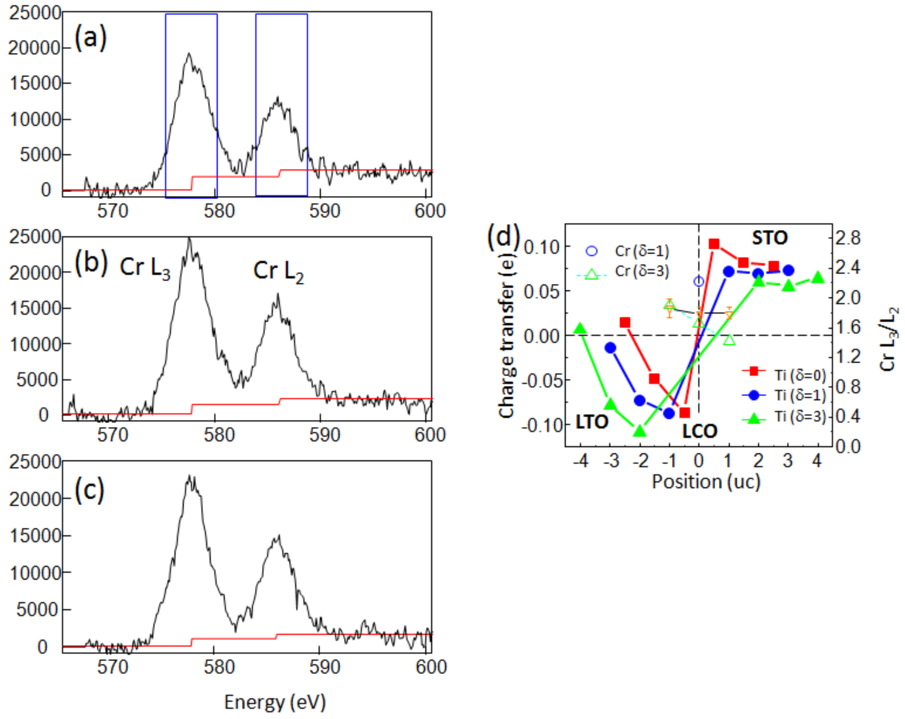


FIG. S7: (a-c) EELS spectra from $LaCrO_3$ layers with (a) to (c) from LTO/LCO interface to LCO/STO interface, showing Cr $L_3$ and $L_2$ edges. The Cr-$L_3$ pre-absorption edge background was subtracted using power law method. The energy is calibrated based on zero loss which is simultaneously acquired using Dual EELS. Cr $L_3$ peak position are measured to be 577.94, 577.9 and 577.8 eV, respectively, indicating possible valence reduction of Cr. To further evaluate the valence state, the Cr $L_3/L_2$ ratio is calculated using the two-step function (method II, red line in the figure) used by Daulton et al [10]. The intensity under the L-edges is measured by integrating 5-eV-wide region centered with respect to the L-edge maximum (blue rectangle in (a)). (d) DFT calculations (Fig. 1(b) in main text) with measured $L_3/L_2$ ratio (brown triangles). Apparently, the $L_3/L_2$ ratio in our films is higher than that of $Cr^{3+}$, confirming reduced valence of Cr in the film.
